# Supplementary material for: Demystifying Compiler Unstable Feature Usage and Impacts in the Rust Ecosystem
Source: arXiv:2310.17186 source file (2023-10-26)
Supplement: Supplementary file 1 [file 9-appendix.tex]

\section{Appendix}

\subsection{Object Explanation}

Due to space limitation, we don't use Rust specific object names in some description.

Package: Packages in this paper are referred to \textit{crates} in Rust. Although, they have slight differences, we don't want to confuse readers into too much detail on that. 

Feature: There are multiple types of \textit{feature} defined in different levels in Rust, but they have different meanings. Cargo has its unstable feature, too. Rust unstable feature is sometimes called Nightly feature.

Dependencies: Names of dependency type in different pakcage managers are different. Development dependencies in NPM are not the same as it in Cargo.

\subsection{Accuracy Evaluation Detail}

As Cargo uses flat structure to store dependency resolution results, we don't define dependency trees as original ones. Instead, we only consider whether we select exact same version as benchmark, rather than comparing the whole dependency chain.

\subsection{RUF extraction evaluation}

\subsection{Dependency Resolution challenges}

\subsection{Extending our tool}

\subsection{Full RUF Impact Definition}
